# Supplementary material for: The Breakdown of Mott Physics at VO$_2$ Surfaces
Source: arXiv:2012.05306 source file (2020-12-09)
Supplement: Supplementary file 1 [file VO2surfaces_supp.pdf]

# The Breakdown of Mott Physics at $VO_2$ Surfaces

Matthew J. Wahila,[1] Nicholas F. Quackenbush,[1] Jerzy T. Sadowski,[2] Jon-Olaf Krisponeit,[3] Jan Ingo Flege,[3,4] Richard Tran,[5] Shyue Ping Ong,[5] Christoph Schlueter,[6] Tien-Lin Lee,[6] Megan E. Holtz,[7] David A. Muller,[7,8] Hanjong Paik,[9] Darrell G. Schlom,[9,8] Wei-Cheng Lee,[1] and Louis F. J. Piper[1,10,a)]

[1)] *Department of Physics, Applied Physics and Astronomy, Binghamton University, Binghamton, New York 13902, USA*

[2)] *Center for Functional Nanomaterials, Brookhaven National Laboratory, Upton, New York 11973, USA*

[3)] *Institute of Solid State Physics, University of Bremen, Otto-Hahn-Allee 1, 28359 Bremen, DE*

[4)] *Applied Physics and Semiconductor Spectroscopy, Brandenburg University of Technology Cottbus-Senftenberg, Konrad-Zuse-Str. 1, 03046 Cottbus, DE*

[5)] *Department of NanoEngineering, University of California San Diego, 9500 Gilman Drive 0448, La Jolla, California 92093, USA*

[6)] *Diamond Light Source Ltd., Diamond House, Harwell Science and Innovation Campus, Didcot, Oxfordshire OX11 0DE, UK*

[7)] *School of Applied and Engineering Physics, Cornell University, Ithaca, NY 14853, USA*

[8)] *Kavli Institute at Cornell for Nanoscale Science, Ithaca, New York 14853, USA*

[9)] *Department of Materials Science and Engineering, Cornell University, Ithaca, New York 14853-1501, USA*

[10)] *Materials Science & Engineering, Binghamton University, Binghamton, New York 13902, USA*

[a]Electronic mail: lpiper@binghamton.edu

## I. TEMPERATURE-DEPENDENT HAXPES/XAS SPECTRA FOR ALL ORIENTATIONS

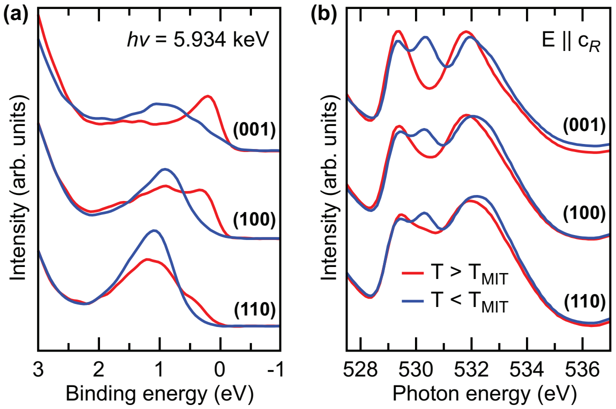


FIG. 1. **(a)** Valence band HAXPES and **(b)** O K-edge XAS of $VO_2/TiO_2$(001), (100), and (110) epitaxial thin films both above and below their respective MIT temperatures.

HAXPES and XAS spectra of all three orientations of $VO_2/TiO_2$ thin films investigated in this study are shown in Figure I. Spectra were taken both above and below the MIT temperatures of each film. Comparing the two spectra reveals the changes to the electronic structure associated with the MIT.

## II. SAMPLE PREPARATION DETAILS

All samples in this study had some minor air exposure as we were unable to grow and characterize the surfaces in-situ. Because of this, extensive care was taken to develop a method to prepare clean and ordered surfaces before the very surface sensitive LEED/LEEM measurements. Generally, only in-situ cleaving of crystals or ion bombardment followed by annealing in oxygen can produce surfaces with sufficient long-range order to reveal a LEED pattern.[1] For $VO_2$ crystals, however, one study found several ordered crystal surfaces at room temperature after simply annealing under an oxygen partial pressure.[2] Based on this method, we were able to observe reasonable LEED patterns on average after 3 anneal cycles under an oxygen partial pressure ($P_{O_2}$) of $1.0 \times 10^{-6}$ Torr, each held for 1 hour at 250 °C. Higher temperatures would be expected to produce cleaner surfaces, however, all anneals had to be performed with restrained heating rates (~5°/min) and a maximum temperature

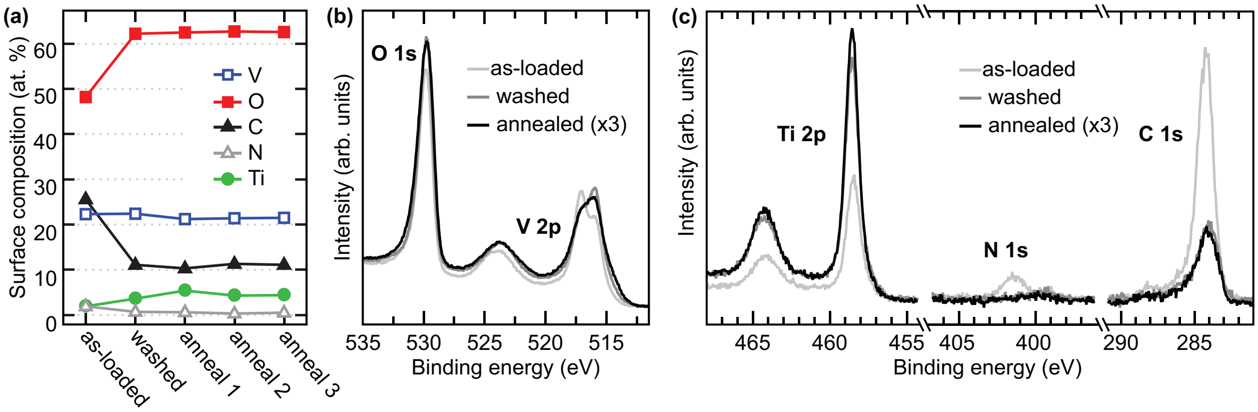


FIG. 2. **(a)** Surface at. % composition measured for a 10 nm $VO_2/TiO_2(001)$ film at each stage of the surface preparation. The corresponding XPS spectra of the **(b)** O 1s and V 2p core levels, and the **(c)** Ti 2p, N 1s, and C 1s core levels at select stages in the process.

of 350 °C in order to avoid diffusion of titanium ions from the substrate into the $VO_2$ film.[3] It was therefore necessary to develop an alternative low-temperature process to prepare our $VO_2$ surfaces before the annealing procedure.

Air exposed $VO_2$ surfaces have been reported to possess a native over-oxidized surface layer.[4] Various etching methods have been pursued in an attempt to remove this layer. Both plasma etching in air and gentle ion bombardment *in-vacuo* were found to reduce the vanadium to a $3^+$ oxidation state. An alternate approach was to chemically etch the $VO_2$ films before introducing them into the experimental chamber, however, all standard etchants tested either over-reduced the $VO_2$ film or removed the film entirely. Surprisingly, we have found that an acetone bath successfully removes the majority of the overlayer without reducing or otherwise damaging the bulk film. The washing procedure was to place the sample for ∼20 seconds in an acetone bath, followed by ∼20 seconds in an isopropanol bath, followed by a rinse with deionized water, and finally the sample was dried using a dry $N_2$ stream. This procedure was successful at producing LEED patterns for each $VO_2$ surface, even before any annealing or other surface preparation steps.

XPS was used to monitor the surface composition at each stage of the surface preparation. Figure 2a shows the compositions by atomic percentage as measured for a 10 nm $VO_2/TiO_2(001)$ film. First, the film was measured as-loaded without washing. Next, the sample was removed from vacuum, washed as described above, and promptly reintroduced to the XPS chamber for measurement. Following this, three anneals were then performed

successively as described above, allowing the sample to cool to room temperature before each XPS measurement. It is clear that the most effective step in removing surface carbon and nitrogen species is the acetone wash, since the composition changes only very slightly after each anneal.

Figures 2b and c show the core level XPS spectra used in the composition analysis. The spectra reveal a large decrease of the $V^{5+}$ upon washing concomitant with an increase in the Ti 2p signal from the substrate. This indicates that the overall thickness of the $VO_2$ film is reduced upon washing, with the $V^{5+}$ surface layer being stripped away along with the carbon and oxygen surface contamination. As such, it is likely that air-exposure of the $VO_2$ surface results in an organic species wherein carbon is strongly bonded to oxidized $V^{5+}$ ions from the film. It is then this organic layer which is effectively stripped away by the acetone wash.

Although our washing and low temperature annealing leave a small amount of residual carbon observable with XPS, we believe these surfaces should still be clean enough to accurately represent $VO_2$. From the C 1s core level intensity observed after washing, we estimate the remaining carbon on the surface to be significantly less than one monolayer of coverage.

## III. POST-LEEM ANALYSIS OF $VO_2$(110) SURFACE OXIDATION

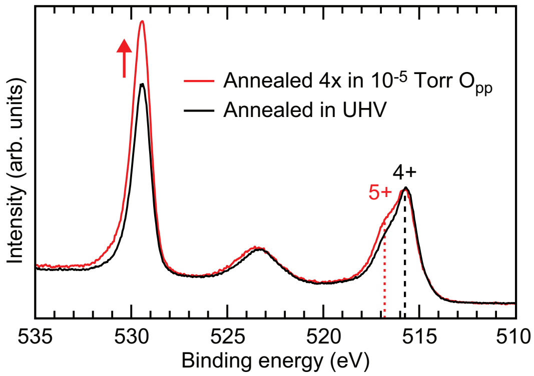


FIG. 3. Core level XPS taken on two $VO_2/TiO_2$(110) films after annealing with and without an oxygen partial pressure.

Post-analysis of two (110) films, shown in Supplementary Figure 3, confirms annealing under a high oxygen partial pressure results in more oxidized $V^{5+}$ and more relative oxygen content. Taken together with the LEED/LEEM, this indicates that the (2×2) reconstruction

it is not related to the bulk MIT, but is instead due to ordered oxygen adsorption on the film surface with a periodicity twice that of the underlying unit cell. Meanwhile, the electron-stimulated desorption of this oxygen and its effects on the LEED/LEEM may help to explain some previous accounts of a "decoupled" transition observed using these very surface sensitive techniques.[5,6] This experiment illustrates why MIT studies must include thorough investigations of reversibility and reproducibility, especially regarding materials like $VO_2$ which are sensitive to beam damage and other complicating effects.

## IV. ALL CALCULATED STRUCTURES FOR $VO_2(110)$ $-1 \leq \Gamma \geq 3$ SLABS

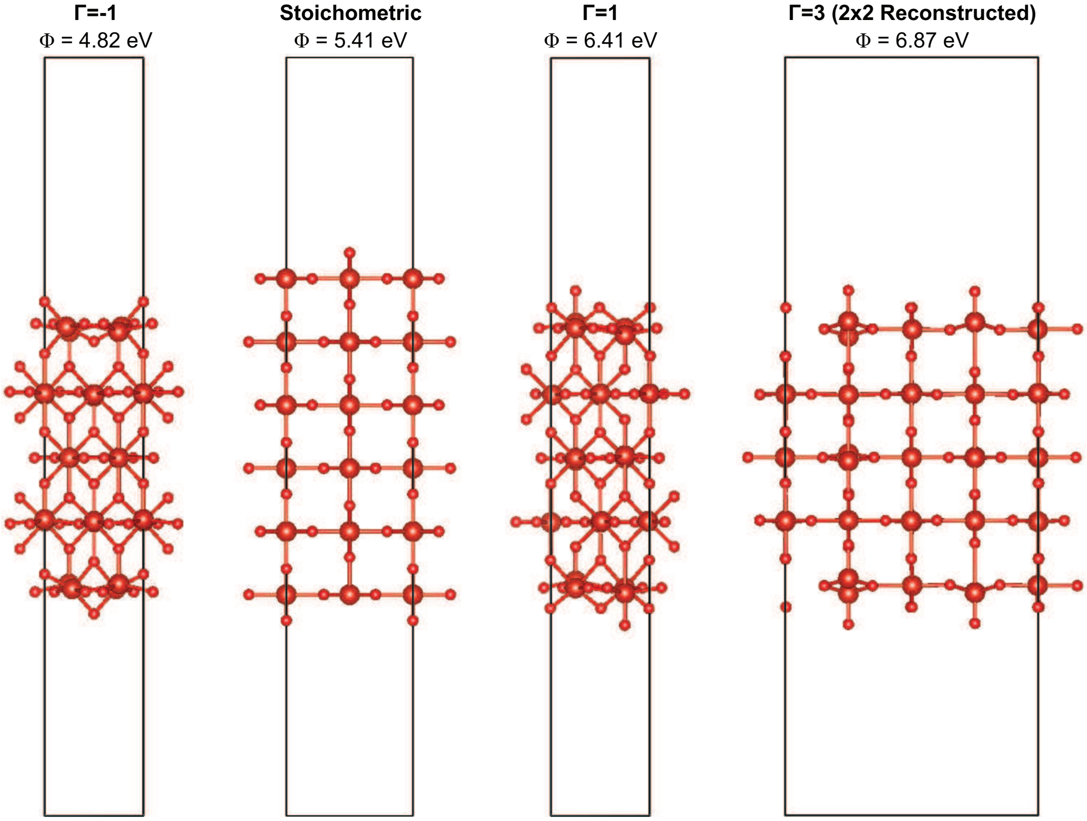


FIG. 4. Reconstructed $VO_2(110)$ rutile slabs predicted for $-1 \leq \Gamma \leq 3$, showing vanadyl bonds on the oxygen rich surfaces.

All slabs shown in Supplementary Figure 4 were generated using the algorithm described by Sun et al.[7] We start by fully relaxing the conventional unit cell of $VO_2$. For each unique Miller index whose surface we investigated, we applied a transformation matrix to the conventional unit cell to obtain an oriented unit cell (OUC) whereby the transformed $\mathbf{a} \times \mathbf{b}$

plane is parallel to the Miller index plane of the surface. We then relax the OUC before constructing a supercell. All slab cells contain a slab and vacuum layer of at least 15Å and were constrained to have symmetric top and bottom surfaces. We constructed our non-stoichiometric slabs (O adsorption/desorption) by symmetrically removing V (adsorption) or O (desorption) atoms on both surfaces.

To construct the (110) $2 \times 2$ reconstruction, we start by quadrupling the surface area our $\Gamma = 3$ (O-saturated) termination (thus quadrupling the slab cell size overall). We then identify all surface O sites and iterated through all possible combinations of O adsorption/desorption on the surface that results in a $2 \times 2$ surface symmetry, thus yielding 16 possible unique reconstructions.

## V. CALCULATED WORK FUNCTIONS FOR THE $(110)_R$ AND $(011)_M$ SURFACES

TABLE I. The calculated work function ($\Phi$) of the corresponding rutile slabs in Supplementary Figure 4 and the stoichiometric monoclinic slab.

| (hkl) | $\Gamma$ | $\Phi$ (eV) |
|---|---|---|
| $(011)_M$ | 0 | 5.59 |
| $(110)_R$ | 0 | 5.41 |
| $(110)_R$ | -1 | 4.82 |
| $(110)_R$ | 1 | 6.41 |
| $(110)_R$ $2 \times 2$ | 3 | 6.87 |

The work function ($\Phi$) for all terminations of the (110) rutile surfaces and the corresponding (011) monoclinic surfaces are shown in Table I. For the rutile phase, we observe a significant increase (0.46 eV to 1 eV) in $\Phi$ as the surface becomes more saturated with oxygen. $\Phi$ decreases slightly by 0.18 eV as $VO_2$ transitions from the rutile to monoclinic phase ($(110)_R \rightarrow (011)_M$.

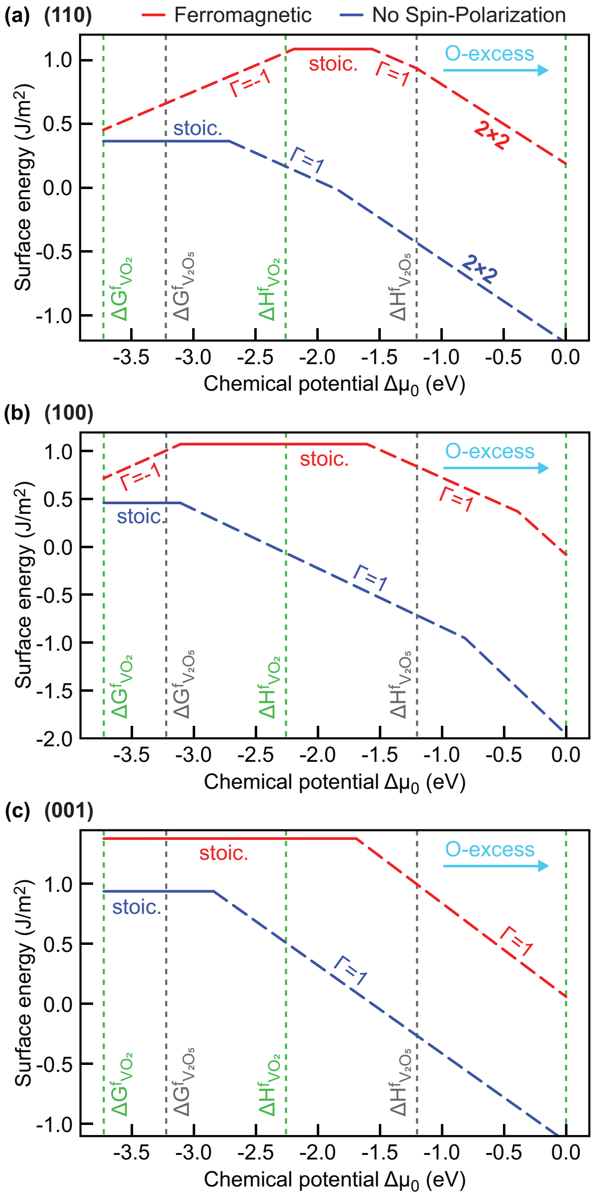


| (110) Ferromagnetic | |
|---|---|
| $\Delta\mu_O$ (eV) | excess/deficient O (Å$^{-2}$) |
| -2.19 | -0.026 |
| -1.56 | 0 |
| -1.22 | 0.026 |
| > | 0.037 |

| (110) No Spin-Pol. | |
|---|---|
| $\Delta\mu_O$ (eV) | excess/deficient O (Å$^{-2}$) |
| -2.71 | 0 |
| -1.83 | 0.027 |
| > | 0.041 |

| (100) Ferromagnetic | |
|---|---|
| $\Delta\mu_O$ (eV) | excess/deficient O (Å$^{-2}$) |
| -3.12 | -0.036 |
| -1.59 | 0 |
| -0.38 | 0.036 |
| > | 0.073 |

| (110) No Spin-Pol. | |
|---|---|
| $\Delta\mu_O$ (eV) | excess/deficient O (Å$^{-2}$) |
| -3.11 | 0 |
| -0.81 | 0.038 |
| > | 0.077 |

| (001) Ferromagnetic | |
|---|---|
| $\Delta\mu_O$ (eV) | excess/deficient O (Å$^{-2}$) |
| -1.69 | 0.049 |
| > | 0 |

| (110) No Spin-Pol. | |
|---|---|
| $\Delta\mu_O$ (eV) | excess/deficient O (Å$^{-2}$) |
| -2.84 | 0 |
| > | 0.046 |

FIG. 5. Predicted surface energy of $VO_2$ as a function of oxygen chemical potential in the **(a)** (110), **(b)** (100), and **(c)** (001) orientations. For context, we drew vertical dashed lines for the formation energy per oxygen atom of $VO_2$ and $V_2O_5$ ($\Delta G^f_{VO_2}$ and $\Delta G^f_{V_2O_5}$) and the enthalpy of reaction for $V_2O_5$ relative to $VO_2$ ($\Delta H^f_{V_2O_5}$).

## VI. CALCULATED SURFACE ENERGIES FOR MAXIMUM MILLER INDICES OF 1

The surface energies plotted in Supplementary Figure 5 can be derived from Equation 1. Here, the chemical potential accounts for atomic species exchanged between the surface and

an external reservoir (i.e. the surrounding environment in the form of a gas, liquid or bulk phase). In the case of the $VO_2$ surfaces, we can expand Equation 1 to:

$$\gamma = \frac{1}{2A}[E^{slab} - N_O\mu_O - N_V\mu_V] \tag{1}$$

To simplify this equation, we assume that the surface phase is in equilibrium with the bulk. Under this assumption, the chemical potential for all species is connected via Gibbs free energy per formula unit[8]:

$$g^{bulk}_{\mathrm{VO_2}} = \sum_i n_i\mu_i = \mu_V + 2\mu_O \tag{2}$$

where $n_i$ is the number of species $i$ in the formula $VO_2$ ($n_V = 1, n_O = 2$). Assuming there is no configurational entropy or pressure-volume effects, $g^{bulk}_{\mathrm{VO_2}}$ can be calculated as the total bulk DFT energy per formula unit. We can therefore rewrite Equation 1 as a function of $\mu_O$ by substituting Equation 2 for $\mu_V$:

$$\gamma = \frac{1}{2A}[E^{slab} - N_V(g^{bulk}_{\mathrm{VO_2}} - 2\mu_O) - N_O\mu_O] \tag{3}$$

A reasonable upper and lower bound is needed for $\mu_O$ to allow for the exchanging of O atoms between the surface and the external reservoir. The upper bound is set by the assumption $O_2$ will saturate the surface while the lower bound is set by the assumption that a surface deficiency of O (or equivalently an excess of V) will lead to the formation of $V_2O_3$ from $VO_2$. This range for $\mu_O$ is expressed as:

$$\Delta G_{\mathrm{VO_2}} \leq \mu_O \leq \frac{1}{2}E_{\mathrm{O_2}} \tag{4}$$

Here $\Delta G_{\mathrm{VO_2}} = -3.74$ eV is the formation energy per oxygen atom and $E_{\mathrm{O_2}}$ is the total DFT energy of molecular $O_2$. Since the bulk $VO_2$ phase is known to decompose via the following reaction:

$$2\,\mathrm{VO_2} + \tfrac{1}{2}\,\mathrm{O_2} \longrightarrow \mathrm{V_2O_5} \tag{5}$$

we can give further context to $\Delta\mu_O$ by indicating the enthalpy of reaction for $V_2O_5$, i.e. the chemical potential in which $VO_2$ is stable relative to $V_2O_5$ which is given by $\Delta H^f_{\mathrm{V_2O_5}} = -1.196$ eV. For convenience, we set the upper bound as a zero reference by subtracting $\frac{1}{2}E_{\mathrm{O_2}}$ from $\mu_O$ leaving us with:

$$\Delta G_{\mathrm{VO_2}} \leq \Delta\mu_O \leq 0 \tag{6}$$

where $\mu_O = \Delta\mu_O + \frac{1}{2}E_{\mathrm{O}_2}$. Substituting our expression for $\mu_O$ into Equation 3 will yield the following expression for surface energy:

$$\gamma = \frac{1}{2A}[E^{slab} - N_V g^{bulk}_{\mathrm{VO}_2} + (2N_V - N_O)(\Delta\mu_O + \frac{1}{2}E_{\mathrm{O}_2})] \tag{7}$$

or:

$$\gamma = \frac{1}{2A}[E^{slab} - N_V g^{bulk}_{\mathrm{VO}_2}] + \Gamma(\Delta\mu_O + \frac{1}{2}E_{\mathrm{O}_2})] \tag{8}$$

where $\Gamma = \frac{1}{2A}(2N_V - N_O)$ is the number of excess ($\Gamma > 0$) or deficient ($\Gamma < 0$) O atoms per surface area (coverage). Note that in a stoichiometric system ($\Gamma = 0$), the surface energy becomes a constant value independent of $\Delta\mu_O$ (see lines labeled "stoic." in Supplementary Figure 5) given by:

$$\gamma = \frac{1}{2A}[E^{slab} - N_V g^{bulk}_{\mathrm{VO}_2}] \tag{9}$$

Since the calculation of surface energies requires the mixing of values determined with ($E^{slab}$ and $g^{bulk}_{\mathrm{O}_2}$) and without ($E_{\mathrm{O}_2}$) the Hubbard-U, we need to apply an anionic correction value to $E_{\mathrm{O}_2}$ in accordance to the Materials Project[9]:

$$E_{\mathrm{O}_2} = E^{uncorr}_{\mathrm{O}_2} + E_{corr} \tag{10}$$

where $E_{corr} = -0.7023$ eV is derived from fitting the calculated formation enthalpy of various V-O compounds with $U = 3.25$ eV to those obtained experimentally.[10] The possible surface coverages of each slab within the chemical potential range of stability for $\mathrm{VO}_2$ are listed in the tables in Supplementary Figure 5.

## VII. MAGNETIC CONSIDERATIONS OF DFT

The monoclinic phase is known to be non-magnetic. We can investigate the surface properties of non-magnetic monoclinic $\mathrm{VO}_2$ by either setting the initial magnetic moments of all atoms to $0\mu_B$ or by omitting spin-polarization. Under the former setting, relaxation of the monoclinic slab structure results in a ferromagnetic slab and a straightening of all vanadium dimers to the characteristic 180° angle associated with the rutile phase. Essentially, the slab no longer corresponds to the non-magnetic monoclinic phase, but instead a ferromagnetic rutile phase. As such, we elect to compare the stoichiometric surface energies and work functions of both phases using a non spin-polarized solution instead.

On the other hand, calculations of non-stoichiometric surface energies for rutile $VO_2$ will yield unphysical negative values as the chemical potential of oxygen increases in the absence of spin-polarization as shown in Supplementary Figure 5. As such we also calculated the ferromagnetic surface energies of rutile $VO_2$ which yields positive surface energies values. Both magnetic configurations demonstrates the same terminations will stabilize under the given chemical potential range. As such, we can interpret the ferromagnetic surface energies when discussing the rutile surfaces only.

## REFERENCES


[1]S. Surnev, M. G. Ramsey, and F. P. Netzer, "Vanadium oxide surface studies," Prog. Surf. Sci. **73**, 117–165 (2003).

[2]E. Goering, M. Schramme, O. Müller, R. Barth, H. Paulin, M. Klemm, M. L. DenBoer, and S. Horn, "LEED and photoemission study of the stability of VO2 surfaces," Phys. Rev. B **55**, 4225–4230 (1997).

[3]N. F. Quackenbush, H. Paik, M. E. Holtz, M. J. Wahila, J. A. Moyer, S. Barthel, T. O. Wehling, D. A. Arena, J. C. Woicik, D. A. Muller, D. G. Schlom, and L. F. J. Piper, "Reducing orbital occupancy in $VO_2$ suppresses Mott physics while Peierls distortions persist," Physical Review B **96**, 081103(R) (2017).

[4]N. F. Quackenbush, H. Paik, J. C. Woicik, D. A. Arena, D. G. Schlom, and L. F. J. Piper, "X-Ray Spectroscopy of Ultra-Thin Oxide/Oxide Heteroepitaxial Films: A Case Study of Single-Nanometer $VO_2$/$TiO_2$," Materials **2**, 5452–5466 (2015).

[5]J. Laverock, S. Kittiwatanakul, a. a. Zakharov, Y. R. Niu, B. Chen, S. a. Wolf, J. W. Lu, and K. E. Smith, "Direct Observation of Decoupled Structural and Electronic Transitions and an Ambient Pressure Monocliniclike Metallic Phase of VO2," Phys. Rev. Lett. **113**, 1–5 (2014).

[6]J. Laverock, V. Jovic, A. A. Zakharov, Y. R. Niu, S. Kittiwatanakul, B. Westhenry, J. W. Lu, S. A. Wolf, and K. E. Smith, "Observation of Weakened V - V Dimers in the Monoclinic Metallic Phase of Strained VO2," Physical Review Letters **121**, 256403 (2018).

[7]W. Sun and G. Ceder, "Efficient creation and convergence of surface slabs," Surface Science **617**, 53–59 (2013).

[8]J. Rogal and K. Reuter, "Ab Initio Atomistic Thermodynamics for Surfaces : A Primer,"

Experiment, Modeling and Simulation of Gas-Surface Interactions for Reactive Flows in Hypersonic Flights , 2–1 – 2–18 (2007).

[9] A. Jain, G. Hautier, S. P. Ong, C. J. Moore, C. C. Fischer, K. A. Persson, and G. Ceder, “Formation enthalpies by mixing GGA and GGA + U calculations,” Physical Review B **84**, 045115 (2011).

[10] L. Wang, T. Maxisch, and G. Ceder, “Oxidation energies of transition metal oxides within the GGA+U framework,” Physical Review B **73**, 195107 (2006), arXiv:9605103 [cs].
